# Supplementary material for: TutteNet: Injective 3D Deformations by Composition of 2D Mesh Deformations
Source: arXiv:2406.12121 source file (2024-06-20)
Supplement: Supplementary file 1 [file X_suppl.tex]

\clearpage
\setcounter{page}{1}
% \vspace{0.3in}
\maketitlesupplementary
\section{Computation of the Jacobian of $\map_\theta$}
\label{sec:jacobian_computation}
The deformation's Jacobian can be computed in a quick and straightforward manner. Let $\p\in\rthree$, and a prismatic map $\layer^i$ defined with respect to $\rotation^i,\planlayer^i$ as in Section~\ref{section:method:representation}. Then the Jacobian of $\layer^i$ at point $\p$ is
\begin{equation}
\label{eq:prism_jac}
    \jac{\layer^i\equiv\rotation^i}{\p} \tilde{A}_\tri {\rotation^i}^T,
\end{equation}
where $\tri$ is the triangle the point lies in (per Algorithm~\ref{alg:point_map}), and
   ${\tilde{A}_\tri = 
\begin{pNiceArray}{cc cc}[small]
    \Block{2-2}{A_\tri} & & 0\\ 
    & & 0 
    \\
    0 &  0 & 1
\end{pNiceArray}}$ is the 2D Jacobian of the 2D mesh deformation at point $\p$, lifted to 3D.
Finally, the Jacobian of the map $\map$ at point $\p$ can be computed by applying the chain rule to equation~\eqref{eq:map}, 
\begin{equation}
\label{eq:map_jac}
    \jac{\map}{\p} = \Pi_{i=o}^n \jac{\layer^i}{\p}.
\end{equation}
\section{Technical details}
\label{sec:tech}
\paragraph{Elastic deformation (Section~\ref{sec:exp:arap}).}

We use a \our{} with 24 layers, each with a mesh of $25\times25$ vertices. We set the local coordinate system $\rotation^i$ of each layer in a triplane manner, alternating between the 3 main axes.
The input shapes are normalized so that all the points are between $[-0.7, 0.7]^3$. We optimize the parameters using Adam~\cite{kingma2014adam} with an initial learning rate of 0.02, with linear decay to 0.0002 in 4000 steps. We set $\weighthandles=1$,  $\weightlayer=0.005$.  We initialize $\weightarap=0.004$, reducing by $0.001$ every 600 steps until reaching $\weightarap=0.001$. 

To evaluate the integrals~\eqref{eq:lossarap},~\eqref{eq:losshandles} we consider only points that exceed a NeRF density $\sigma\parr{p}>1$, and from them uniformly sample 10K points from user-selected handles that change location, 15K points from handles that are chosen to remain static, and 10k points from the remaining set, i.e., ones on the part to be deformed.  To accelerate reduction of distortion, at regions where distortion (Equation~\eqref{eq:arap_energy}) reaches $>0.02$, we multiply the weight on $\lossarap$ by 2, and at areas with distortion $>0.05$, we multiply the weight by 5.

\paragraph{Fitting (Section~\ref{sec:exp:comparisons})}
 Our \our{} has 24 layers set in a triplane manner, as above. Each layer uses meshes with $11\times11$ vertices. 
We optimize using Adam~\cite{Adam} with an initial learning rate of 0.02, linearly decaying to 0.002 in 5000 steps.

\paragraph{Learning (Section~\ref{sec:exp:learn})}

The \our{} is composed of 24 Tutte layers, with each layer having a mesh with $11\times11$ vertices. The local coordinate frames $\rotation^i$ are not fixed, but also predicted by the network.

To predict the deformation parameters $\theta^i$ of each prismatic layer $\layer^i$, we construct three networks to predict the three deformation parameters, the laplacian $\lap^i$, the boundary locations $\bdry^i$, and the coordinate frame $\rotation^i$ (refer to Section~\ref{section:method:representation} and Figure~\ref{fig:diagram}). 

Both $\lap^i$ and $\bdry^i$ assign one scalar to each edge or a vertex (respectively) of the 2D mesh $\mesh$. We use the same architecture to predict each of them: we leverage the geometric nature of the mesh, feeding each vertex concatenated with $\z$ into the network, which predicts a scalar for that vertex. Similarly, for the edges, we input the midpoint $m_{ij}$ of each edge $\parr{i,j}$. We represent each input using a positional encoding with a basis of size $50$. 

For the prediction of the local coordinate frame $\rotation^i$, we have an MLP predict the unit-norm normal $\bm{n}_3$ of the projection plane of the Tutte layer, we complete it to an orthonormal system via $\bm{n}_1 = \bm{n}_3\times \parr{0,0,1}$, $\bm{n}_2 = \bm{n}_3 \times \bm{n}_1$.

All three networks are residual MLPs. For the $\lap$ and $\bdry$ MLPs we use a 512-channel linear layer, followed by 3 512-channel residual blocks, for the $\rotation$ MLP we use a 256-channel linear layer followed by 2 256-channel residual blocks.

Each of these three networks predicts parameters for all the prismatic layers simultaneously, their output being a tensor with one entry for each primsatic map $\layer^i$.

Lastly, to encode the input human shapes, we generate depth-image renderings from 8 different views and feed them to image encoders, CLIP\cite{clip} and DINO-V2\cite{dinov2},  to get feature vectors, which we then feed to a 3-layer MLP with hidden layers of width $\brac{1025,512,256}$.

% \section{Rationale}
% \label{sec:rationale}
% % 
% Having the supplementary compiled together with the main paper means that:
% % 
% \begin{itemize}
% \item The supplementary can back-reference sections of the main paper, for example, we can refer to \cref{sec:intro};
% \item The main paper can forward reference sub-sections within the supplementary explicitly (e.g. referring to a particular experiment); 
% \item When submitted to arXiv, the supplementary will already included at the end of the paper.
% \end{itemize}
% % 
% To split the supplementary pages from the main paper, you can use \href{https://support.apple.com/en-ca/guide/preview/prvw11793/mac#:~:text=Delete%20a%20page%20from%20a,or%20choose%20Edit%20%3E%20Delete).}{Preview (on macOS)}, \href{https://www.adobe.com/acrobat/how-to/delete-pages-from-pdf.html#:~:text=Choose%20%E2%80%9CTools%E2%80%9D%20%3E%20%E2%80%9COrganize,or%20pages%20from%20the%20file.}{Adobe Acrobat} (on all OSs), as well as \href{https://superuser.com/questions/517986/is-it-possible-to-delete-some-pages-of-a-pdf-document}{command line tools}.

\paragraph{$K$-plane representation.}

Our representation could be seen as a type of $K$-plane method. $K$-planes, and especially triplanes, have two particularly attractive properties for representing 3D volumetric data : (1) compactness and (2) the ability to leverage 2D techniques for 3D tasks by treating each plane as an image. In ConvOccNet, Peng et al.~\cite{convolutionaloccnet}  project 3D point features on planes and apply U-Nets on each plane to perform a 3D reconstruction.  EG3D~\cite{gao2022get3d} introduces a 3D GANs based on an efficient novel architecture that queries features on a triplane representation and processes them with a small MLP head. Their representation serves as the basis for several follow-up generative techniques based on GANs~\cite{gao2022get3d, wu2022learning, deng20233d, sun2022ide} and diffusion~\cite{nfd, gupta20233dgen, gaudi}. Similarly to EG3D, TensorRF~\cite{tensorf} proposes to factorize the 3D tensors of NeRFs using triplanes, drastically speeding up reconstruction and novel view rendering. Their triplane representation was extended to anti-aliased NeRF renderings~\cite{trimiprf}, spatio-temporal radiance fields~\cite{dtensorf, tensor4d, kplanes_2023, hexplane}, surface reflectance reconstruction~\cite{tensoir} and occupancy prediction~\cite{huang2023tri}. In contrast to these methods, in TutteNet, we leverage $K$-planes to represent \textit{3D deformation}. The triplane representation also enables us to leverage an established 2D technique, Tutte embeddings.%, by applying it on each plane and composing them.

% First papers to democratize it
% Convolutional Occupancy Network~\cite{convolutionaloccnet} introduces a more-memory efficient triplane representation decode occupancy grids. 
% EG3D~\cite{eg3d}

% Nerfs and 4D nerfs
% TensoRF~\cite{tensorf} represents the volumetric density and radiance via vector-matrix outer products,
% Tri-mipRF~\cite{trimiprf} extends it to anti-aliased renderings.
% TensoIR~\cite{tensoir} extends to estimate surface reflectance and environment illumination.
% K-planes~\cite{kplanes_2023} extends to spatiotemporal volumes with 6-plane decomposition. 
% Tensor4D~\cite{tensor4d} uses 9 planes.
% D-Tensorf~\cite{dtensorf}. 
% Hexplane~\cite{hexplane} use 6 planes, extented to a generated settings in MAV3D~\cite{singer2023text4d} (diffusion)
% \cite{huang2023tri} autonomous driving application of tri-plane occupancy prediction from RGB images.

% Generative
%% GANS
% EG3D~\cite{eg3d} use a triplane-representation for 3D GANs, by querying features aligned on three orthogonal planes, and passing them to a small MLP head. 
% Get3D~\cite{gao2022get3d} follow-up on arbitrary categories, also triplane. 
% \cite{wu2022learning} generative 3D with Gans ans triplane.
% Pix2Pix3D~\cite{deng20233d} 3D generative models with triplanes.
% \cite{sun2022ide} more generative stuff. 

%% Diffusion
% NFD~\cite{nfd} introduces tri-plane diffusion to leverage recent advancements in 2D diffusion for 3D generation. 
% \cite{gupta20233dgen} also introduces triplane diffusion.
% Gaudi~\cite{gaudi} generative radiance field with triplanes for interiors.
